# Supplementary material for: Linear Last-iterate Convergence in Constrained Saddle-point Optimization
Source: arXiv:2006.09517 source file (2021-03-19)
Supplement: Supplementary file 1 [file appendix-J.tex]

\section{Proofs of \pref{thm:sg arbitrary}}
\begin{proof}[Proof of Theorem~\ref{thm:arbitrary}]
     By Lemma~\ref{lem: value difference}, for any $x$, 
     \begin{align}
          \rho_{x_t, y_t} - \rho_{x, y_t} = \sum_{s\in\calS} \mu^s_{x, y_t}   \left(x^s_t - x^s\right)^\top Q^s_{t,t} y_t^s. \label{eq:value_diff_lemma} 
     \end{align}
     Note that $\left(x^s_t - x^s\right)^\top Q^s_{t,t} y_t^s$ is essentially the instantaneous regret of \alg on the state $s$ at episode $t$. By \pref{eq: sg regret one side}, we have %the same analysis as in \pref{lem: regret bound} (specifically \pref{eq: to be continue 1} and \pref{lem: proj optimal}), we have 
     \begin{align}
          (x^s_t - x^s_*)^\top Q^s_{t,t} y^s_t   % \nonumber 
          %&\leq \frac{\|x^s_* - \xp^s_t\|^2  - \|x^s_* - \xp^s_{t+1}\|^2}{2\eta} + \left(x_t^s - \xp_{t+1}^s\right)^\top \left(Q_{t,t}^s y_t^s - Q_{t, t-1}^s y_{t-1}^s\right)    \nonumber \\
          &\leq \frac{\|x^s_* - \xp^s_t\|^2  - \|x^s_* - \xp^s_{t+1}\|^2}{2\eta} + \eta\|Q^s_{t,t} y^s_t - Q^s_{t,t-1} y^s_{t-1}\|^2.  \label{eq: regret bound for x sg}
     \end{align}
     By \pref{lem:Q diff lemma}, for $t\geq 2$, 
     \begin{align}
          &\|Q^s_{t,t} y^s_t - Q^s_{t,t-1} y^s_{t-1}\|^2  \nonumber  \\
          &\leq 2 \|Q^s_{t,t} \left(y^s_t - y^s_{t-1}\right)\|^2 + 2\|\left(Q^s_{t,t} - Q^s_{t,t-1}\right) y^s_{t-1}\|^2 \nonumber \\
          &\leq 2H^2 A \|y^s_t-y^s_{t-1}\|_1^2 + 2H^2 A \left(\sum_{i=h+1}^H \max_{s'\in\calS_i}  \|y^{s'}_t - y^{s'}_{t-1}\|_1\right)^2 \tag{By \pref{lem:Q diff lemma}; $A\triangleq |\calA|$}  \nonumber \\
          &\leq 2H^2 A \Theta_{t,h}^2 + 2H^3 A \sum_{i=h+1}^H  \Theta_{t,i}^2    \tag{$\Theta_{t,h} \triangleq \max_{s\in\calS_h }\|y_t^s-y_{t-1}^s\|_1$},
          &\label{eq: stability term sg 2}
          %&\leq 2H^2 AB \|y_s^t-y_s^{t-1}\|^2 + 2H^3 A \sum_{i=h+1}^H \max_{s'\in\calS_i} \|y_{s'}^t - y_{s'}^{t-1}\|_1^2
          %&\leq 2H^2 AB \|y_s^t-y_s^{t-1}\|^2 + 2H^3 AB \sum_{i=h+1}^H \max_{s'\in\calS_i} \|y_{s'}^t - y_{s'}^{t-1}\|^2 \\
          %&\leq 2H^2 AB \|y_s^t-y_s^{t-1}\|^2 + 2H^3 AB \sum_{i=h+1}^H \sum_{s'\in\calS_i}  \|y_{s'}^t - y_{s'}^{t-1}\|^2
     \end{align}
     where in the last step we use Cauchy-Schwarz inequality.
     Also, for $t=1$, $\|Q^s_{t,t} y^s_t - Q^s_{t,t-1} y^s_{t-1}\|^2= O(H^2A)$. 
     Plugging these bounds into \pref{eq: regret bound for x sg}, we have for any $h$, 
     \begin{align*}
          &\sum_{t=1}^T \sum_{s\in\calS_h} \mu^s_{x_*, y_t} (x^s_t - x^s_*)^\top Q^s_{t,t} y^s_t \\
          &\leq \sum_{t=1}^T \sum_{s\in\calS_h} \frac{\mu^s_{x_*, y_t} \|x^s_*-\xp^s_t\|^2 - \mu^s_{x_*, y_t}\|x^s_*-\xp^s_{t+1}\|^2}{2\eta} + \sum_{t=2}^T \left(2\eta H^2 A\Theta_{t,h}^2 + 2\eta H^3 A \sum_{i=h+1}^H \Theta_{t,i}^2\right) \\ 
          &\qquad\qquad + O\left(\eta H^2A\right)  \tag{$\sum_{s\in\calS_h} \mu^s_{x_*, y_t}=1$} \\
          &\leq \sum_{t=2}^T \sum_{s\in\calS_h} \frac{\|x^s_*-\xp^s_t\|^2 \left( \mu^s_{x^*, y_t} - \mu^s_{x^*, y_{t-1}} \right)}{2\eta} + \sum_{t=1}^T \left(2\eta H^2 A\Theta_{t,h}^2 + 2\eta H^3 A \sum_{i=h+1}^H \Theta_{t,i}^2\right) \\
          &\qquad\qquad + O\left( \frac{\sum_{s\in\calS_h} \mu^s_{x_*, y_1}}{\eta} + \eta H^2A \right) \\
          &\leq 2\sum_{t=2}^T \sum_{s\in\calS_h} \frac{\left\vert \mu^s_{x_*, y_t} - \mu^s_{x_*, y_{t-1}} \right\vert}{\eta} + \sum_{t=2}^T \left(2\eta H^2 A\Theta_{t,h}^2 + 2\eta H^3 A \sum_{i=h+1}^H \Theta_{t,i}^2\right) + O\left(\frac{1}{\eta}+\eta H^2A\right)\\
          &\leq 2\sum_{t=2}^T \sum_{i=1}^{h-1} \frac{  \Theta_{t,i}  }{\eta} + \sum_{t=2}^T \left(2\eta H^2 A\Theta_{t,h}^2 + 2\eta H^3 A \sum_{i=h+1}^H \Theta_{t,i}^2\right) + O\left(\frac{1}{\eta}+\eta H^2A\right).  \tag{by \pref{lem:mu decompose}}
     \end{align*}
     Finally summing over $h$ and combining with \pref{eq:value_diff_lemma} we have
     \begin{align*}
          &\sum_{t=1}^T \left(\rho_{x_t, y_t} - \rho_{x_*, y_t}\right) \\
          & \leq  2\sum_{t=2}^T \sum_{h=1}^H \sum_{i=1}^{h-1} \frac{  \Theta_{t,i}  }{\eta} + \sum_{t=2}^T \left(2\eta H^2 A \sum_{h=1}^H \Theta_{t,h}^2 + 2\eta H^3 A \sum_{h=1}^H \sum_{i=h+1}^H \Theta_{t,i}^2\right) + O\left(\frac{H}{\eta}+\eta H^3A\right)\\
          &= O\left(\frac{H}{\eta}\sum_{t=2}^T \sum_{h=1}^H \Theta_{t,h} +  \eta H^4 A \sum_{t=2}^T \sum_{h=1}^H  \Theta_{t,h}^2 \right) + O\left(\frac{H}{\eta}+\eta H^3A\right),
     \end{align*}
     completing the proof.
\end{proof}
