# Supplementary material for: Linear Last-iterate Convergence in Constrained Saddle-point Optimization
Source: arXiv:2006.09517 source file (2021-03-19)
Supplement: Supplementary file 2 [file appendix-part2.tex]

%!TEX root=iclr2021_conference.tex

\section{Auxiliary Lemmas for Stochastic Games}

\begin{definition}\label{def:stationary distribution}
     Define $\mu^s_{x,y}$ as the probability of visiting state $s$ given that the players use policies $(x,y)$. By the game structure, it satisfies the following:  
     \begin{align*}
          &\mu^{s'}_{x,y} = 
          \begin{cases}
               p_0(s')  &\text{if\ } s'\in\calS_1,  \\
               \sum_{s\in\calS} \sum_{a,b} x^{s}(a) y^{s}(b) p(s'~|~s,a,b) \mu^{s}_{x,y}   &\text{if\ } s'\notin \calS_1. 
          \end{cases}
     \end{align*}
     Also, $\sum_{s\in\calS_h}\mu^s_{x,y}=1$ for any $h, x, y$. 
\end{definition}

\begin{lemma}[Value difference lemma]\label{lem: value difference}
For any policies $x, y, \xtil, \ytil$, we have
\begin{align*}
     \rho_{x,y} - \rho_{\xtil,\ytil} = \sum_{s\in\calS}\sum_{a,b} \mu^s_{\xtil,\ytil} \Big(x^{s}(a)y^{s}(b)- \xtil^s(a)\ytil^s(b)\Big) Q_{x,y}^s(a,b). 
\end{align*}
\end{lemma}
\begin{proof}
By definitions, we have the following equalities:
    \begin{align*}
          \rho_{\xtil, \ytil} 
          &= \sum_{s\in\calS} \sum_{a,b} \mu^s_{\xtil, \ytil}  \xtil^{s}(a) \ytil^{s}(b) \ell(s,a,b) \\
          &= \sum_{s\in\calS} \sum_{a,b} \mu^s_{\xtil, \ytil}  \xtil^{s}(a)\ytil^{s}(b) \left(Q^s_{x,y}(a,b) - \sum_{s'\in\calS} p(s'~|~s,a,b) V^{s'}_{x,y} \right)   \tag{by the definition of $Q_{x,y}^s$} \\
          &= \sum_{s\in\calS} \sum_{a,b} \mu^s_{\xtil, \ytil}  \xtil^{s}(a)\ytil^{s}(b) Q^s_{x,y}(a,b) - \sum_{s'\in\calS\backslash \calS_1} \mu^{s'}_{\xtil,\ytil} V^{s'}_{x,y}    \tag{by \pref{def:stationary distribution}}\\
          &= \sum_{s\in\calS} \sum_{a,b} \mu^s_{\xtil, \ytil}  \xtil^{s}(a)\ytil^{s}(b) Q^s_{x,y}(a,b) - \sum_{s\in\calS} \mu^{s}_{\xtil,\ytil} V^{s}_{x,y} + \sum_{s\in\calS_1} \mu^s_{\xtil, \ytil} V^s_{x,y} \\
          &= \sum_{s\in\calS} \sum_{a,b} \mu^s_{\xtil, \ytil}  \Big(\xtil^{s}(a)\ytil^{s}(b) - x^s(a)y^s(b) \Big)Q^s_{x,y}(a,b) + \sum_{s\in\calS_1} p_0(s) V^s_{x,y} \tag{by the definition of $V_{x,y}^s$} \\
          &= \sum_{s\in\calS} \sum_{a,b} \mu^s_{\xtil, \ytil}  \Big(\xtil^{s}(a)\ytil^{s}(b) - x^s(a)y^s(b) \Big)Q^s_{x,y}(a,b) + \rho_{x,y}.
          %&= \sum_{s\in\calS} \sum_{a,b} \mu_s^{x, y^t}  \left(x_s(a)-x_s^t(a)\right) y^t_s(b) Q_s^{t,t}(a,b) + \rho^{x^t, y^t} \\
          %&= \sum_{s\in\calS} \mu_s^{x, y^t}  \left(x_s-x_s^t\right)^\top Q_s^{t,t} y^t_s + \rho^{x^t, y^t}.
     \end{align*}
     Rearranging the above finishes the proof. 
\end{proof}

\begin{lemma}
    \label{lem:Q diff lemma}
    Let $s\in\calS_h$ for some $h$. Then for any actions $a,b$ and any policies $x, y, \xtil, \ytil$, we have
    \begin{align*}
         \left\vert Q^s_{\xtil,\ytil}(a,b) - Q^s_{x,y}(a,b)\right\vert 
         &\leq H \left( \sum_{i=h+1}^H \max_{s'\in\calS_i} \|\xtil^{s'} - x^{s'}\|_1 + \|\ytil^{s'} - y^{s'}\|_1 \right).
         %&\leq H^2\sqrt{A+B} \max_{i>h, s'\in \calS_i} \left(\|\xtil^{s'}-x^{s'}\| + \|\ytil^{s'}-y^{s'}\|\right).
    \end{align*}
\end{lemma}

\begin{proof}
    Notice that for $s\in\calS_i$, by definition we have 
    \begin{align*}
         \left\vert Q^s_{\xtil,\ytil}(a,b) - Q^s_{x,y}(a,b)\right\vert 
         &\leq \sum_{s'} p(s'~|~s,a,b) \left\vert V^{s'}_{\xtil,\ytil} - V^{s'}_{x,y}\right\vert \\
         &\leq \max_{s'\in\calS_{i+1}} \left\vert V^{s'}_{\xtil,\ytil} - V^{s'}_{x,y}\right\vert
    \end{align*}
    and 
    \begin{align*}
         &\left\vert V^s_{\xtil, \ytil} - V^s_{x, y} \right\vert \\
         &=\left\vert \sum_{a, b}  \xtil^{s}(a) \ytil^{s}(b) Q^s_{\xtil,\ytil}(a,b) -  \sum_{a, b}x^s(a) y^s(b) Q^s_{x,y}(a,b) \right\vert\\
         &\leq \sum_{a, b} \left\vert  \xtil^{s}(a) \ytil^{s}(b) Q^s_{\xtil,\ytil}(a,b) -  x^s(a) y^s(b) Q^s_{x,y}(a,b) \right\vert\\
         &\leq \sum_{a, b} \left\vert  \xtil^{s}(a)-x^s(a) \right\vert \ytil^{s}(b) Q^s_{\xtil,\ytil}(a,b) \\
         & \qquad + \sum_{a,b} x^s(a) \left\vert  \ytil^s(b) - y^s(b) \right\vert Q^s_{\xtil,\ytil}(a,b) \\
         &\qquad  + \sum_{a,b} x^s(a)y^s(b) \left\vert Q^s_{\xtil,\ytil}(a,b) - Q^s_{x,y}(a,b)\right\vert \\
         %&=  \sum_{a, b} \left(x'_s(a) y'_s(b) Q_s^{x',y'}(a,b) -  x_s(a) y'_s(b) Q_s^{x',y'}(a,b)\right) \\
         %&  \qquad+ \sum_{a, b} \left(x_s(a) y'_s(b) Q_s^{x',y'}(a,b) -  x_s(a) y_s(b) Q_s^{x',y'}(a,b)\right) \\
         %& \qquad = \sum_{a, b} \left(x_s(a) y_s(b) Q_s^{x',y'}(a,b) -  x_s(a) y_s(b) Q_s^{x,y}(a,b)\right) \\
         &\leq H\|\xtil^s-x^s\|_1 + H\|\ytil^s-y^s\|_1 + \sum_{a,b}x^s(a)y^s(b) \left\vert Q^s_{\xtil, \ytil}(a,b)-Q^s_{x,y}(a,b)\right\vert \\
         &\leq H\|\xtil^s-x^s\|_1 + H\|\ytil^s-y^s\|_1 + \max_{a,b} \left\vert Q^s_{\xtil, \ytil}(a,b)-Q^s_{x,y}(a,b)\right\vert,
    \end{align*}
    where in the second to last step we use the fact that $Q^s_{x,y}(a,b)$ is at most $H$ clearly.
    Using the above two relations repeatedly for $i=h,h+1,\dots,H-1$ proves the result. 
\end{proof}

\begin{corollary}\label{corr: Qy}
     For any $y'\in\Delta_\calB$, $s \in \calS_h$ for some $h$, $z=(x,y)$, and $\ztil=(\xtil, \ytil)$, we have
     \begin{align*}
          &\| (Q^s_{x,y}-Q^s_{\xtil, \ytil})y' \|_\infty \leq H^2 \sqrt{A+B}\max_{i>h, s'\in\calS_i} \|\ztil^{s'}-z^{s'}\|, \\
          &\| (Q^s_{x,y}-Q^s_{\xtil, y})y' \|_\infty \leq H^2 \sqrt{A}\max_{i>h, s'\in\calS_i} \|\xtil^{s'}-x^{s'}\|, \\
          &\| (Q^s_{x,y}-Q^s_{x, \ytil})y' \|_\infty \leq H^2 \sqrt{B}\max_{i>h, s'\in\calS_i} \|\ytil^{s'}-y^{s'}\|, 
     \end{align*} 
     where $A = |\calA|$, $B = |\calB|$ and $\|\cdot\|$ is 2-norm.
\end{corollary}
\begin{proof}
The first inequality can be shown by the following:
     \begin{align*}
          &\| (Q^s_{x,y}-Q^s_{\xtil, \ytil})y' \|_\infty  \\
          &= \max_i \left\vert \e_i^\top (Q^s_{x,y}-Q^s_{\xtil, \ytil})y' \right\vert \\
          &= \max_i \left\| \e_i^\top (Q^s_{x,y}-Q^s_{\xtil, \ytil}) \right\|_\infty \|y'\|_1 \\
          &\leq H \left( \sum_{i=h+1}^H \max_{s'\in\calS_i} \|\xtil^{s'} - x^{s'}\|_1 + \|\ytil^{s'} - y^{s'}\|_1 \right) \tag{by \pref{lem:Q diff lemma}}\\
          &\leq H^2 \max_{i>h, s'\in\calS_i} \sqrt{A}\|\xtil^{s'}-x^{s'}\| + \sqrt{B}\|\ytil^{s'}-y^{s'}\| \\
          &\leq H^2 \sqrt{A+B}\max_{i>h, s'\in\calS_i} \|\ztil^{s'}-z^{s'}\| \tag{Cauchy-Schwarz inequality}. 
     \end{align*}
     The other two inequalities can be obtained similarly. 
\end{proof}

\begin{lemma}
     \label{lem:mu decompose}
     For any $h$ and any polices $x, y, \xtil, \ytil$, we have
     \begin{align*}
         \sum_{s'\in\calS_h}\left\vert \mu^{s'}_{\xtil,\ytil} - \mu^{s'}_{x,y} \right\vert \leq \sum_{i=1}^{h-1}\left( \max_{s\in\calS_i} \|\xtil^s-x^s\|_1 + \max_{s\in\calS_i} \|\ytil^s-y^s\|_1\right).  
     \end{align*}
\end{lemma}
\begin{proof}
By \pref{def:stationary distribution}, we proceed with
    \begin{align*}
         &\sum_{s'\in\calS_h}\left\vert \mu^{s'}_{\xtil,\ytil} - \mu^{s'}_{x,y} \right\vert  \\
         &=\sum_{s'\in\calS_h} \left\vert \sum_{s\in\calS_{h-1}} \sum_{a,b} \left(\xtil^s(a)\ytil^s(b) p(s'~|~s,a,b) \mu^{s}_{\xtil,\ytil} -  x^s(a) y^s(b) p(s'~|~s,a,b) \mu^{s}_{x,y}\right) \right\vert \\
         &\leq \sum_{s\in\calS_{h-1}} \sum_{a,b}\left(\sum_{s'\in\calS_h} p(s'~|~s,a,b)\right) \left\vert \left(\xtil^s(a)\ytil^s(b)  \mu^{s}_{\xtil,\ytil} -  x^s(a) y^s(b) \mu^{s}_{x,y}\right) \right\vert \\
         &= \sum_{s\in\calS_{h-1}} \sum_{a,b} \left\vert  \xtil^s(a) \ytil^s(b) \mu^{s}_{\xtil,\ytil} -  x^s(a) y^s(b)\mu^{s}_{x,y} \right\vert  \\
         &\leq \sum_{s\in\calS_{h-1}} \sum_{a,b} \left\vert \xtil^s(a) - x^s(a) \right\vert \ytil^s(b)\mu^s_{\xtil, \ytil} \
          +  \sum_{s\in\calS_{h-1}} \sum_{a,b}  x^s(a) \left\vert \ytil^s(b) - y^s(b) \right\vert \mu^s_{\xtil, \ytil}  \\
          &\quad\quad +  \sum_{s\in\calS_{h-1}} \sum_{a,b} x^s(a)y^s(b) \left\vert  \mu^s_{\xtil, \ytil} - \mu^s_{x,y}  \right\vert  \\
         &\leq \max_{s\in\calS_{h-1}}\|\xtil^s-x^s\|_1 + \max_{s\in\calS_{h-1}}\|\ytil^s-y^s\|_1 + \sum_{s\in\calS_{h-1}} \left\vert \mu^s_{\xtil,\ytil} - \mu^s_{x,y}\right\vert.
    \end{align*}
    Applying the above inequality repeatedly finishes the proof. 
\end{proof}

\section{Proofs of \pref{thm:sg last iterate}}
We follow our convention that $z^s\triangleq (x^s, y^s)$. Also, we define the following notation: 
\begin{definition}
     Define $\Phi_{t,h} = \max_{i\geq h}\max_{s\in\calS_i} \|z^s_t-z^s_*\|^2$. 
\end{definition}

\begin{lemma}\label{lem: sufficient decrease sg}
     For any $s \in \calS_h$ and any $\ztil^s=(\xtil^s, \ytil^s)$ such that $\left(\xp_{t+1}^{s^\top} Q_{*}^s \ytil^s - \xtil^{s^\top} Q_{*}^s \yp_{t+1}^{s}\right) > 0$,  we have
     \begin{align*}
          \|z_t^s- \zp_t^s\|^2 + \|\zp_{t+1}^s-z_{t}^s\|^2 \geq \frac{64}{1875}\eta^2\left(\xp_{t+1}^{s^\top} Q_{*}^s \ytil^s - \xtil^{s^\top} Q_{*}^s \yp_{t+1}^{s}\right)^2 - H^2 \Phi_{t,h+1}. 
     \end{align*}
\end{lemma}
\begin{proof}
     The proof follows similar arguments of the proof of \pref{lem: sufficient decrease}.  By the optimality of $\xp_{t+1}^s$ we have for any $\xtil^s$, 
     \begin{align*}
          &(\xp_{t+1}^s-\xp_{t}^s + \eta Q_{t,t}^s y_t^s)^\top (\xtil^s - \xp_{t+1}^s)\geq 0. 
     \end{align*}
     Rearranging, we get 
     \begin{align}\label{eq: tmptmp}
         (\xp_{t+1}^s-\xp_{t}^s)^\top (\xtil^s - \xp_{t+1}^s)  \geq \eta  (\xp_{t+1}^s-\xtil^s)Q_{t,t}^s y_t^s.
     \end{align}
     Because $\|\xtil^s - \xp_{t+1}^s\|\leq 2$, for the left-hand side we have $(\xp_{t+1}^s-\xp_{t}^s)^\top (\xtil^s - \xp_{t+1}^s)  \leq 2\|\xp_{t+1}^s - \xp_t^s\|$. For the right-hand side, we have 
    \begin{align*}
        &\eta  (\xp_{t+1}^s-\xtil^s)^\top Q_{t,t}^s y_{t}^s\\
        &=\eta (\xp_{t+1}^s-\xtil^s)^\top Q_{*}^s \yp_{t+1}^s + \eta(\xp_{t+1}^s-\xtil^s)^\top (Q_{t,t}^s - Q_*^s)\yp_{t+1}^s + \eta(\xp_{t+1}^s-\xtil^s)^\top Q_{t,t}^s (y_t^s - \yp_{t+1}^s) \\
        &\geq \eta (\xp_{t+1}^s-\xtil^s)^\top Q_{*}^s \yp_{t+1}^s - \eta\|\xp_{t+1}^s-\xtil^s\|_1 \|(Q_{t,t}^s - Q_*^s)\yp_{t+1}^s\|_\infty - \eta\|\xp_{t+1}^s-\xtil^s\|_1 \|Q_{t,t}^s  (y_t^s - \yp_{t+1}^s)\|_\infty \\
        &\geq \eta (\xp_{t+1}^s-\xtil^s)^\top Q_{*}^s \yp_{t+1}^s - 2\eta H^2 \sqrt{A+B} \sqrt{\Phi_{t,h+1}}
        - 2\eta H\|y_t^s - \yp_{t+1}^s\|_1
           \tag{using \pref{corr: Qy}}\\
        &\geq \eta (\xp_{t+1}^s-\xtil^s)^\top Q_{*}^s \yp_{t+1}^s - 2\eta H^2 \sqrt{A+B} \sqrt{\Phi_{t,h+1}}
        - 2\eta H\sqrt{B}\|y_t^s - \yp_{t+1}^s\|.
    \end{align*}
    Therefore, with \pref{eq: tmptmp}, we have 
    \begin{align*}
        &2\|\xp_{t+1}^s - \xp_t^s\| + 2\eta H^2 \sqrt{A+B} \sqrt{\Phi_{t,h+1}} + 2\eta H\sqrt{B}\|y_t^s - \yp_{t+1}^s\| \\
        &\geq \eta (\xp_{t+1}^s-\xtil^s)^\top Q_{*}^s \yp_{t+1}^s. 
    \end{align*}
    Similarly for $y$ we can obtain
        \begin{align*}
        &2\|\yp_{t+1}^s - \yp_t^s\| + 2\eta H^2 \sqrt{A+B} \sqrt{\Phi_{t,h+1}} + 2\eta H\sqrt{A}\|x_t^s - \xp_{t+1}^s\| \\
        &\geq \eta \xp_{t+1}^{s^\top} Q_{*}^s (\ytil^s - \yp_{t+1}^s). 
    \end{align*}
    
    Summing up these two inequalities we get 
    \begin{align*}
         &\eta \left( \xp_{t+1}^{s^\top} Q^s_* \ytil^s - \xtil^{s^\top } Q^s_* \yp_{t+1}^s   \right)  \\
         &\leq 2\sqrt{2}\|\zp^s_{t+1}-\zp^s_t\| + 2\eta H\sqrt{2AB}\|z_t^s - \zp_{t+1}^s\| 
         + 4\eta H^2 \sqrt{A+B} \sqrt{\Phi_{t,h+1}} \tag{Cauchy-Schwarz inequality}\\
         &\leq 3\|\zp^s_{t+1}-\zp^s_t\| + 2\eta H\sqrt{2AB}\|z_t^s - \zp_{t+1}^s\| 
          + 4\eta H^2 \sqrt{2AB} \sqrt{\Phi_{t,h+1}} \tag{$2AB\ge A+B$}\\
         &\leq 3\|\zp^s_{t+1}-\zp^s_t\| + \frac{1}{8}\|z_t^s - \zp_{t+1}^s\| + \frac{H}{4} \sqrt{\Phi_{t,h+1}} \tag{$\eta \leq \frac{1}{16H\sqrt{2AB}}$}\\
         &\leq 3\|z_t^s-\zp^s_t\| + \frac{25}{8}\|z_t^s - \zp_{t+1}^s\| + \frac{H}{4} \sqrt{\Phi_{t,h+1}}.
    \end{align*}
    Squaring both sides and using $(a+b+c)^2 \leq 3(a^2+b^2+c^2)$, we get 
    \begin{align*}
         &\eta^2 \left( \xp_{t+1}^{s^\top} Q^s_* \ytil^s - \xtil^{s^\top } Q^s_* \yp_{t+1}^s   \right)^2\\
         &\leq \frac{1875}{64}\left(\|z_t^s-\zp^s_t\|^2 + \|z_t^s - \zp_{t+1}^s\|^2\right) + \frac{3H^2}{16} \Phi_{t,h+1}. 
    \end{align*} 
    Rearranging finishes the proof. 
\end{proof}

\begin{proof}[Proof of \pref{thm:sg last iterate}]
    Consider a state $s\in\calS_h$. By the same analysis as in \pref{lem: regret bound} (specifically \pref{eq: to be continue 1} and \pref{lem: proj optimal}), we have 
     \begin{align}
          &2\eta (x^s_t - x^s_*)^\top Q^s_{t,t} y^s_t \nonumber  \\
          %&\leq \frac{\|x^s_* - x^s_t\|^2  - \|x^s_* - x^s_{t+1}\|^2}{2\eta} + \left(x_t^s - \xp_{t+1}^s\right)^\top \left(Q_{t,t}^s y_t^s - Q_{t, t-1}^s y_{t-1}^s\right)  - \frac{\|\xp_{t+1}^s-x_t^s\|^2 + \|x_t^s-\xp_t^s\|^2}{2\eta}    \nonumber \\
          &\leq \|x^s_* - \xp^s_t\|^2  - \|x^s_* - \xp^s_{t+1}\|^2 + 2\eta^2\|Q^s_{t,t} y^s_t - Q^s_{t,t-1} y^s_{t-1}\|^2 - \|\xp_{t+1}^s-x_t^s\|^2 - \|x_t^s-\xp_t^s\|^2.    \label{eq: sg regret one side}
     \end{align}
     We proceed with
     \begin{align}
          &2\eta^2 \|Q^s_{t,t} y^s_t - Q^s_{t,t-1} y^s_{t-1}\|^2   \nonumber  \\
          &\leq 4\eta^2 \|Q^s_{t,t} \left(y^s_t - y^s_{t-1}\right)\|^2 + 4\eta^2\|\left(Q^s_{t,t} - Q^s_{t,t-1}\right) y^s_{t-1}\|^2 \nonumber \\
          &\leq 4\eta^2 H^2 A \|y^s_t-y^s_{t-1}\|_1^2 + 4\eta^2 A H^4 B \max_{i>h, s'\in\calS_i} \|y_t^{s'}-y_{t-1}^{s'}\|^2 \tag{By \pref{corr: Qy}}  \\
          &\leq 4\eta^2 H^2 AB \|y^s_t-y^s_{t-1}\|^2 + 8\eta^2 H^4 AB (\Phi_{t-1, h+1} + \Phi_{t,h+1})    \nonumber  \\
          &\leq \frac{1}{128} \|y^s_t-y^s_{t-1}\|^2 + \frac{H^2}{64}\left(\Phi_{t-1,h+1}+\Phi_{t,h+1}\right)   \nonumber  \tag{$\eta \leq \frac{1}{16H\sqrt{2AB}}$}\\
          &\leq \frac{1}{64} \|y^s_t-\yp^s_{t}\|^2 + \frac{1}{64} \|\yp_{t}^s - y^s_{t-1}\|^2 + \frac{H^2}{64}\left(\Phi_{t-1,h+1}+\Phi_{t,h+1}\right).   \label{eq: sg stability one side}
     \end{align}
     We can get the $y$ counterpart of \pref{eq: sg regret one side} and \pref{eq: sg stability one side} similarly. Combining all these inequalities leads to
     \begin{align}
         &2\eta (x^s_t - x^s_*)^\top Q^s_{t,t} y^s_t + 2\eta x_t^{s^\top} Q^s_{t,t} (y^s_* - y^s_t )   \nonumber \\
         &\leq \|z_*^s-\zp_t^s\|^2 - \|z_*^s-\zp_{t+1}^s\|^2 + \frac{1}{64}\|\zp_t^s - z_{t-1}^s\|^2 - \frac{63}{64}\|z_t^s- \zp_t^s\|^2 - \|\zp_{t+1}^s-z_{t}^s\|^2 \nonumber \\
         &\qquad + \frac{H^2}{32}\left(\Phi_{t-1, h+1}+ \Phi_{t, h+1}\right)\nonumber \\
         %&\leq \|z_*^s-z_t^s\|^2 - \|z_*^s-z_{t+1}^s\|^2 + \frac{1}{32}\|\zp_t^s - z_{t-1}^s\|^2 - \frac{31}{32}\|z_t^s- \zp_t^s\|^2 - \|\zp_{t+1}^s-z_{t}^s\|^2 + \frac{H^2}{16}\left(\Phi_{t-1, h+1}+ \Phi_{t, h+1}\right)\nonumber \\
         &\leq \|z_*^s-\zp_t^s\|^2 - \|z_*^s-\zp_{t+1}^s\|^2 + \frac{1}{64}\|\zp_t^s - z_{t-1}^s\|^2 - \frac{31}{64}\|\zp_{t+1}^s - z_{t}^s\|^2 \nonumber\\
         & \qquad - \frac{1}{2} \times \frac{64\eta^2 }{1875} \max_{\xtil, \ytil} \left(\xp_{t+1}^{s^\top} Q_{*}^s \ytil^s - \xtil^{s^\top} Q_{*}^s \yp_{t+1}^{s}\right)^2 + \frac{1}{2}H^2\Phi_{t,h+1}  + \frac{H^2}{16}\left(\Phi_{t-1, h+1}+ \Phi_{t, h+1}\right)   \tag{\pref{lem: sufficient decrease sg}}\\
         &\leq \|z_*^s-\zp_t^s\|^2 - \|z_*^s-\zp_{t+1}^s\|^2 + \frac{1}{64}\|\zp_t^s - z_{t-1}^s\|^2 - \frac{31}{64}\|\zp_{t+1}^s - z_{t}^s\|^2 \nonumber\\
         & \qquad - \frac{32\eta^2 C^2}{1875} \|\zp_{t+1}^s-z_*^s\|^2 + H^2\left(\Phi_{t-1, h+1}+ \Phi_{t, h+1}\right). \tag{by \pref{thm: bilinear-polytope} for some constant $C$}\\
          \label{eq: tmp sum sg}
     \end{align}
     
     Note that the left-hand side of \pref{eq: tmp sum sg} can be lower bounded as below: 
     \begin{align*}
         &2\eta (x^s_t - x^s_*)^\top Q^s_{t,t} y^s_t + 2\eta x_t^{s^\top} Q^s_{t,t} (y^s_* - y^s_t)   \\
         &=2\eta (x^s_t - x^s_*)^\top Q^s_{*} y^s_t + 2\eta x_t^{s^\top} Q^s_{*} (y^s_* - y^s_t) \\
         &\qquad + 2\eta (x^s_t - x^s_*)^\top (Q^s_{t,t} - Q^s_{*}) y^s_t + 2\eta x_t^{s^\top} (Q^s_{t,t} - Q^s_{*} )(y^s_* - y^s_t) \\
         &\geq 2\eta (x^s_t - x^s_*)^\top (Q^s_{t,t} - Q^s_{*}) y^s_t + 2\eta x_t^{s^\top} (Q^s_{t,t} - Q^s_{*} )(y^s_* - y^s_t) \tag{by optimality of $x_*^s$ and $y_*^s$}\\
         &\geq -2\eta \|x^s_t - x^s_*\| \|(Q^s_{t,t} - Q^s_{*}) y^s_t\| - 2\eta \|x_t^{s^\top} (Q^s_{t,t} - Q^s_{*})\|\|y^s_* - y^s_t\| \tag{Cauchy-Schwarz inequality}\\
         &\geq - \frac{\eta^2C^2}{1000}\|x^s_t-x^s_*\|^2 - \frac{1000}{C^2}\|(Q^s_{t,t} - Q^s_{*}) y^s_t\|^2 - \frac{\eta^2C^2}{1000}\|y_t^s - y_*^s\|^2 - \frac{1000}{C^2} \|(Q^s_{t,t} - Q^s_*)^\top x_*^s\|^2 \tag{AM-GM inequality} \\
         &\geq -\frac{\eta^2 C^2}{1000} \|z_t^s - z_*^s\|^2 - \frac{1000}{C^2}\times H^4(A+B)^2 \Phi_{t,h+1}    \tag{by \pref{corr: Qy}}\\
         &\geq -\frac{\eta^2 C^2}{500} \|\zp_{t+1}^s - z_*^s\|^2 - \frac{\eta^2 C^2}{500} \|z_{t}^s - \zp_{t+1}^s\|^2 - \frac{1000}{C^2}\times H^4(A+B)^2 \Phi_{t,h+1}.
     \end{align*}
     Combining with \pref{eq: tmp sum sg}, we get 
     \begin{align*}
          \|\zp_{t+1}^s - z_*^s\|^2 
          &\leq \|\zp_{t}^s - z_*^s\|^2 + \frac{1}{64}\|\zp_t^s - z_{t-1}^s\|^2 - \frac{15}{32} \|\zp_{t+1}^s - z_t^s\|^2 - \frac{28\eta^2 C^2}{1875}\|\zp_{t+1}^s - z_*^s\|^2  \\ 
          & \qquad \qquad + \frac{1001H^4(A+B)^2}{C^2}\left(\Phi_{t-1, h+1} + \Phi_{t,h+1}\right). 
     \end{align*}
     Without loss of generality, we assume $C\le 1$ (otherwise we can choose $C=1$). By rearranging terms, we have 
     \begin{align*}
          \|\zp_{t+1}^s - z_*^s\|^2 + \frac{14}{32} \|\zp_{t+1}^s - z_t^s\|^2 &\leq \|\zp_{t+1}^s - z_*^s\|^2 + \frac{15}{32}\cdot \frac{1}{1+\frac{28}{1875}\eta^2 C^2} \|\zp_{t+1}^s - z_t^s\|^2\\
          &\leq \frac{1}{1+\frac{28}{1875}\eta^2 C^2}\left( \|\zp_{t}^s - z_*^s\|^2 + \frac{1}{64} \|\zp_t^s - z_{t-1}^s\|^2 \right) \\
          &\qquad + \frac{1001H^4(A+B)^2}{C^2}\left(\Phi_{t-1, h+1} + \Phi_{t,h+1}\right). 
     \end{align*}
     Note that the above holds for any $z_*^s \in \calZ_*^s$. We choose $z_*^s = \Pi_{\calZ_*^s} (\zp_{t}^s)$. 
     In the following, we use the notation $\Omega_{t}^s = \|\zp_t^s - \Pi_{\calZ_*^s}(\zp_t^s)\|^2$ and $\theta^s_{t} = \|\zp_t^s - z_{t-1}^s\|^2$.  
     Using the fact $\|\zp_{t+1}^s - \Pi_{\calZ_*^s}(\zp_{t+1}^s)\|\leq  \|\zp_{t+1}^s - \Pi_{\calZ_*^s}(\zp_{t}^s)\|$, the above implies
     \begin{align*}
          \Omega^s_{t+1} + \frac{7}{16}\theta^s_{t+1} &\leq \frac{1}{1+\frac{28}{1875}\eta^2 C^2}\left( \Omega_t^s + \frac{7}{16}\theta^s_t \right) \\
          &+ \frac{1001\times 32H^4(A+B)^2}{7C^2}\left[\max_{i> h, s'\in\calS_{i}} \left(\Omega_{t+1}^{s'} + \frac{7}{16}\theta_{t+1}^{s'}\right) + \max_{i> h, s'\in\calS_{i}} \left(\Omega_{t}^{s'} + \frac{7}{16}\theta_{t}^{s'}\right) \right]
     \end{align*}
     because $\Phi_{t,h} = \max_{i\geq h, s'\in\calS_i}\|z_t^{s'}-z_*^{s'}\|^2 \leq  \max_{i\geq h, s'\in\calS_i}\left(2\|z_t^{s'}-\zp_{t+1}^{s'}\|^2 + 2\|\zp_{t+1}^{s'} - z^{s'}_*\|^2\right) = 2\max_{i\ge h, s'\in\calS_i} \left(\Omega_{t+1}^{s'} + \theta_{t+1}^{s'}\right) \leq \frac{32}{7}\max_{i\ge h, s'\in\calS_i} \left(\Omega_{t+1}^{s'} + \frac{7}{16}\theta_{t+1}^{s'}\right)$, where we choose $z_*^{s'}=\Pi_{\calZ_*^{s'}} (\zp_{t+1}^{s'})$.

Below we further define $\zeta_{t,h}\triangleq \max_{s\in\calS_h} \left(\Omega_t^s + \frac{7}{16}\theta_{t}^s\right)$. Then we can further write
\begin{align}
    \zeta_{t+1,h} \leq \frac{\zeta_{t,h}}{1+\frac{28}{1875}\eta^2 C^2} + \frac{5000H^4(A+B)^2}{C^2}\left(\max_{i> h}\zeta_{t+1,i} + \max_{i> h}\zeta_{t,i}\right).    \label{eq: recursion sg}
\end{align}
We use induction to prove that 
\begin{align}\label{eq: recursion to prove sg}
     \zeta_{t,h} \leq 2\left(\frac{1}{1+\frac{1}{1000}\eta^2 C^2}\right)^{t-1} \left(\frac{2\times 10^6H^4(A+B)^2}{\eta^2 C^4}\right)^{H-h}.
\end{align}
It is clear that $t=1$ holds for every layer $h$. 
\paragraph{The last layer. } If $h=H$, then the recursion \pref{eq: recursion sg} implies, for all  $t\in[T]$, 
\begin{align*}
     \zeta_{t, h} \leq 2\left(\frac{1}{1+\frac{28}{1875}\eta^2 C^2}\right)^{t-1} \leq 2\left(\frac{1}{1+\frac{1}{1000}\eta^2 C^2}\right)^{t-1}. 
\end{align*}
\paragraph{Previous layers. } Suppose that the \pref{eq: recursion to prove sg} holds for layers $h+1,\ldots, H$ and for all $t$, and suppose that it holds for time $1,\ldots, t$ for layer $h$. Then by \pref{eq: recursion sg}, 
\begin{align*}
     \zeta_{t+1,h} 
     &\leq \frac{2}{1+\frac{28}{1875}\eta^2 C^2} \left(\frac{1}{1+\frac{1}{1000}\eta^2 C^2}\right)^{t-1} \left(\frac{2\times 10^6H^4(A+B)^2}{\eta^2 C^4}\right)^{H-h} \\
     &\qquad \qquad + \frac{20000H^4(A+B)^2}{C^2} \times \left(\frac{1}{1+\frac{1}{1000}\eta^2 C^2}\right)^{t-1} \times \left(\frac{2\times 10^6H^4(A+B)^2}{\eta^2 C^4}\right)^{H-h-1} \\
     &= \frac{2}{1+\frac{28}{1875}\eta^2 C^2} \left(\frac{1}{1+\frac{1}{1000}\eta^2 C^2}\right)^{t-1} \left(\frac{2\times 10^6H^4(A+B)^2}{\eta^2 C^4}\right)^{H-h} \\
     &\qquad \qquad + \frac{\eta^2 C^2}{100} \times \left(\frac{1}{1+\frac{1}{1000}\eta^2 C^2}\right)^{t-1} \times \left(\frac{2\times 10^6H^4(A+B)^2}{\eta^2 C^4}\right)^{H-h} \\
     &\leq 2\left(\frac{1}{1+\frac{1}{1000}\eta^2 C^2}\right)^{t} \left(\frac{2\times 10^6H^4(A+B)^2}{\eta^2 C^4}\right)^{H-h}\tag{$C<1$}, 
\end{align*}
which finishes the induction. 

Note that \pref{eq: recursion to prove sg} implies that 
\begin{align*}
    \Omega^s_t 
    \leq \zeta_{t, h} &\leq 2\left(\frac{1}{1+\frac{1}{1000}\eta^2 C^2}\right)^{t-1-(H-h) \left( \log \frac{2\times 10^6H^4(A+B)^2}{\eta^2 C^4}\right) \Big/ \left(\log \left(1+\frac{1}{1000}\eta^2 C^2\right)\right)}  \\
    &\leq \left(\frac{1}{1+\frac{1}{1000}\eta^2 C^2}\right)^{t - O\left(\frac{H-h}{\eta^2 C^2} \log \frac{HAB}{\eta C}\right)}, 
\end{align*}
which leads to the desired inequality. 
\end{proof}
