# Supplementary material for: Linear Last-iterate Convergence in Constrained Saddle-point Optimization
Source: arXiv:2006.09517 source file (2021-03-19)
Supplement: Supplementary file 3 [file appendix_unbounded.tex]

\section{\rsi in a Local Region (for unbounded $\calZ$ case)} \label{app: unbounded}
A global $C$ in \pref{def:rsi} might be unavailable in some cases, e.g., bilinear games on an unbounded polyhedron. A sharp contrast is that for any bilinear game on polytopes, one can always find a $C>0$ such that \pref{def:rsi} holds with $\beta=0$ (this is shown by \pref{thm: bilinear-polytope}). To see why it fails to an unbounded polyhedron, suppose that there exists a $C>0$ for a bilinear game $f(\x, \y)=\x^\top \G\y$ in an unbounded polyhedron. Since $\max_{\z'\in\calZ}\frac{F(\z)^\top (\z-\z')}{\|\z-\z'\|} \leq \|F(\z)\|\leq 2\opnorm{G}$ always holds by H\"{o}lder's inequality, as long as we pick some $\z$ such that $\|\z-\Pi_{\calZ^*}(\z)\| > \frac{2\opnorm{G}}{C}$, \rsi fails to hold on this $\z$ with $\beta=0$. 

To handle this case, we note that to argue the convergence rate, what we actually need is only that \rsi holds for all $\{\zp_t\}_{t=1,2,\ldots}$, but not other points (this will be clear in the proof of \pref{thm: point convergence}). More precisely, we only need the following hold: 
\begin{align}
     \sup_{\z'\in\calZ} \frac{F(\z)^\top (\z-\z')}{\|\z-\z'\|} \geq C\|\z-\Pi_{\calZ^*}(\z)\|^{\beta+1}    \label{eq: restricted rsi}
\end{align}
for $\z=\zp_1, \zp_2, \ldots$. 

Below, we will show that there exists bounded regions $\Omega_1\subset\Omega_2\subseteq \calZ$ such that
\begin{enumerate}
\item $\{\zp_t\}_{t=1,2,\ldots}\subset \Omega_1$
\item $\Omega_2^*\subseteq \calZ^*$, where $\Omega^*=\left\{\z\in \Omega:~ F(\z)^\top (\z-\z')\leq 0 \ \ \forall \z'\in \Omega\right\}$ is the set of equilibrium of the game restricted on $\Omega$. 
\end{enumerate}

If the above two properties can be shown, then 
\begin{align*}
     \sup_{\z'\in\Omega_2} \frac{F(\z)^\top (\z-\z')}{\|\z-\z'\|} \geq C\|\z-\Pi_{\Omega_2^*}(\z)\|^{\beta+1} \ \ \forall \z\in\Omega  \Longrightarrow \text{\pref{eq: restricted rsi} holds for $\z=\zp_1, \zp_2, \ldots$}
\end{align*}
because $\sup_{\z'\in\calZ} \frac{F(\z)^\top (\z-\z')}{\|\z-\z'\|} \geq \sup_{\z'\in\Omega} \frac{F(\z)^\top (\z-\z')}{\|\z-\z'\|}$ and $\|\z-\Pi_{\Omega^*}(\z)\|\geq \|\z-\Pi_{\calZ^*}(\z)\|$ (by the second argument above). In other words, to ensure that \pref{eq: restricted rsi} holds for $\z=\zp_1, \zp_2, \ldots$, we only need that \rsi holds for $\Omega$. 
\major{
It remains to prove the existence of such $\Omega$. 
We first show that $\{\zp_t\}_{t=1,2,\ldots}$ indeed lie in a bounded region. By \pref{lem: regret bound omwu} with $\z = \Pi_{\calZ^*}(\zp_1)$, we get 
\begin{align*}
     \norm{\z_{\tau+1} - \Pi_{\calZ^*}(\zp_1)}^2 \leq \norm{\z_{\tau} - \Pi_{\calZ^*}(\zp_1)}^2 - \norm{\zp_{\tau+1} - \z_{\tau}}^2 - \tfrac{15}{16}\norm{\z_{\tau}-\zp_{\tau}}^2 + \tfrac{1}{16}\norm{\zp_{\tau}-\z_{\tau-1}}^2
\end{align*}
for all $\tau \geq 1$. Summing the above inequality from $\tau=1$ to $\tau=t-1$ and performing telescoping, we get 
\begin{align*}
     \norm{\zp_{t} - \Pi_{\calZ^*}(\zp_1)}^2 \leq \norm{\zp_{1} - \Pi_{\calZ^*}(\zp_1)}^2 + \tfrac{1}{16}\norm{\zp_1-\z_0}^2 =  \norm{\zp_{1} - \Pi_{\calZ^*}(\zp_1)}^2. 
\end{align*}

In other words, $\zp_t$ always lies in a ball centered at $\Pi_{\calZ^*}(\zp_1)$ with radius $\norm{\zp_{1} - \Pi_{\calZ^*}(\zp_1)}$, which is a bounded region that depends on the initial point $\zp_1$. Thus, by defining
\begin{align*}
     \Omega=\left\{\z\in\calZ: ~ \|\z-\Pi_{\calZ^*}(\zp_1)\| \leq \|\zp_1 - \Pi_{\calZ^*}(\zp_1)\|\right\}. 
\end{align*}
we can ensure the first property described above. Next, we show that the second property also holds. Suppose that $\z\in\calZ \backslash \calZ^*$, that is, 
\begin{align*}
    \exists \z'\in \calZ, \quad F(\z)^\top (\z-\z') > 0. 
\end{align*}

Based on the discussions above, we only need that all $\z\in\calZ\cap \Omega$ satisfy \rsi. Therefore, for the case of bilinear games in an unbounded polyhedron, we can easily construct a bounded polytope that contains $\calZ\cap \Omega$. Then by \pref{thm: bilinear-polytope}, \rsi holds for all points in this region. Then finally by \pref{thm: point convergence}, we can also argue linear convergence for bilinear games on unbounded polyhedrons. 
}
