# Supplementary material for: Linear Last-iterate Convergence in Constrained Saddle-point Optimization
Source: arXiv:2006.09517 source file (2021-03-19)
Supplement: Supplementary file 4 [file appendix_bilinear_backup.tex]

%!TEX root=neurips_2020.tex

\section{Proof of \pref{thm: bilinear-polytope}}
\label{app:bilinear polytope}

\begin{proof}[Proof of \pref{thm: bilinear-polytope}]
	Let $\rho = \min_{x\in\calX}\max_{y\in\calY} x^\top G y = \max_{y\in\calY}\min_{x\in\calX} x^\top G y$ be the game value. In this proof, our goal is to show that for any $y\notin\calY^*$, then
	\begin{align}
	\max_{x'\in\calX} \frac{\rho-x^{\prime \top }Gy }{\|y-\Pi_{\calY^*}(y)\|} \geq C \label{eq: lower bound of duali}
	\end{align}
	for some constant $C>0$.
	By the exact same analysis one also has 
		\begin{align*}
	\max_{y'\in\calX} \frac{x^\top Gy' - \rho}{\|x-\Pi_{\calX^*}(x)\|} \geq C,
	\end{align*}
	and combining the two proves that for all $z' \in \calZ$,
	\[F(z)^\top (z-z') = x^\top Gy' - x^{\prime \top }Gy \geq C\left(\|y-\Pi_{\calY^*}(y)\| + \|x-\Pi_{\calX^*}(x)\|\right) \geq C\|z-\Pi_{\calZ^*}(z)\|,\] meaning that \typeone holds with $\beta=0$. 
	
	We will in fact prove the following  result that is stronger than \pref{eq: lower bound of duali}: 
      \begin{align}
	\max_{x'\in \calV^*(\calX)} \frac{\rho-x^{\prime \top }Gy }{\|y-\Pi_{\calY^*}(y)\|} \geq C>0    \label{eq: stronger lower bound}
	\end{align}
	where $\calV^*(\calX)$ is a subset of the vertices of $\calX$. To formally define $\calV^*(\calX)$, we let 
	     $\calV(\calX) = \{w_1, w_2, \ldots, w_{|\calV(\calX)|}\}$ be the set of all vertices of $\calX$.	
	Then $\calV^*(\calX)$ is defined as follows: 
	\begin{align*}
	     \calV^*(\calX)\triangleq \left\{w_i\in\calV(\calX): \exists x^*\in\calX^* \text{\ s.t. } x^*=\sum_{i=1}^{|\calV(\calX)|} p_j w_j, \sum_{j=1}^{|\calV(\calX)|}p_j=1, ~ p_i > 0, ~ p_j\geq 0,  ~ \forall j\neq i \right\}. 
	\end{align*}
	In other words, $\calV^*(\calX)$ is the set of vertices $w_i$ for which there exists a minimax optimal solution $x^*$ such that $x^*$ can be written as a convex combination of $\calV(\calX)$ with a positive weight from $w_i$. We  define $\calV(\calY)$ and $\calV^*(\calY)$ similarly. 
	
	We now claim the following fact, which is a consequence of the first statement of \pref{lem: deffered lemma} (by swaping the roles of $x$ and $y$ there). 
	\begin{align}
	     \max_{x'\in\calV^*(\calX)} \frac{\rho-x^{\prime \top }Gy }{\|y-\Pi_{\calY^*}(y)\|} = \max_{x'\in\calV^*(\calX) } \frac{x^{\prime \top} G(\Pi_{\calY^*}(y)-y) }{\|y-\Pi_{\calY^*}(y)\|}.    \label{eq: deffered bound}
	\end{align}
     We first prove that \pref{eq: deffered bound} is positive when $y\notin \calY^*$. It suffices to prove that 
     \begin{align}
          \max_{x'\in\calV^*(\calX)}x^{\prime \top} G(\Pi_{\calY^*(y)}-y) > 0.  \label{eq: statement 1}
     \end{align}
	If $y$ can be decomposed into convex combination of $\calV(\calY)$ with positive weights from $\calV(\calY)\backslash \calV^*(\calY)$, then by the second statement of \pref{lem: deffered lemma}, there exists $x^*\in\calX^*$ such that $x^{* \top}Gy < \rho$. Because $x^*$ is a convex combination of $\calV^*(\calX)$ (by the definition of $\calV^*(\calX)$), we have $x^{*\top}G\Pi_{\calY^*}(y)=\rho$ by the first statement of \pref{lem: deffered lemma}. Therefore, $x^{*\top}G(\Pi_{\calY^*}(y)-y)>0$. Again, since $x^*$ is a convex combination of $\calV^*(\calX)$, this implies that $\max_{x'\in\calV^*(\calX)}x^{\prime\top}G(\Pi_{\calY^*}(y)-y) > 0$, further implying that \pref{eq: statement 1} holds. 
Now suppose that $y$ is a convex combination of $\calV^*(\calY)$, and suppose that \pref{eq: statement 1} does not hold. Then we have 
$
	      \max_{x'\in\calV^*(\calX)} x^{\prime\top}G(\Pi_{\calY^*}(y)-y) \leq 0. 
$
This implies that $y\in\calY^*$, contradicting that $y\notin \calY^*$.
	
	Having shown that \pref{eq: deffered bound} is positive for any $y\notin\calY^*$. Below we show that it is lower bounded by a positive value. 
	Define 
	\begin{align*}
	\Phi_{\calY} \triangleq \left\{y-\Pi_{\calY^*}(y): y\in \calY\right\}
	\end{align*}
	and the conical extension of $\Phi_\calY$: 
	\begin{align*}
	 \mathcal{C}(\Phi_\calY) \triangleq \left\{rv: v\in\Phi_\calY, r\geq 0\right\}.  
	\end{align*}
	Now we prove that $\mathcal{C}(\Phi_\calY) \cap \{v: \|v\|=1\} = \left\{\frac{y-\Pi_{\calY^*}(y)}{\|y-\Pi_{\calY^*}(y)\|}: y\in \calY\backslash \calY^* \right\}$. 
	\ \\
	``$\supseteq$'': Let $v=\frac{y-\Pi_{\calY^*}(y)}{\|y-\Pi_{\calY^*}(y)\|}$ for some $y\in\calY\backslash \calY^*$. Then clearly, $\|v\|=1$, and since $v=r(y-\Pi_{\calY^*}(y))$ with $r=\frac{1}{\|y-\Pi_{\calY^*}(y)\|}$, we also have $v\in\mathcal{C}(\Phi_\calY)$. \\
	``$\subseteq$'': Let $\|v\|=1$ and $v\in\mathcal{C}(\Phi_\calY)$. Then we can express $v$ as $r(y-\Pi_{\calY^*}(y))$ for some $y\in\calY$ and $r\geq 0$. Since $v\neq 0$, $x$ must not be in $\calY^*$. To satisfy $\|v\|=1$, $r$ has to be $\frac{1}{\|y-\Pi_{\calY^*}(x)\|}$. Therefore, $v\in \left\{\frac{y-\Pi_{\calY^*}(y)}{\|y-\Pi_{\calY^*}(y)\|}: y\in \calY\backslash \calY^* \right\}$. 
	
	Next consider the following set of real numbers: 
	\begin{align*}
	\mathcal{S}=\left\{ \max_{x'\in\calV^*(\calX)} \frac{ x^{\prime\top} G(\Pi_{\calY^*}(y)-y)}{\|y-\Pi_{\calY^*}(y)\|}: \quad y\in \calY\backslash \calY^* \right\}. 
	\end{align*}
	All elements of $\mathcal{S}$ are positive by our previous arguments. We can also write $\mathcal{S}$ as 
	\begin{align*}
	\mathcal{S} = \left\{ \max_{x'\in\calV^*(\calX)} x^{\prime\top} G(-v): v\in\mathcal{C}(\Phi_\calY) \text{\ and\ } \|v\|=1 \right\}. 
	\end{align*}
	In this expression, the elements in $\mathcal{S}$ are expressed as function values of a continuous function on the set $\mathcal{C}(\Phi) \cap \{v: \|v\|=1\}$. 
	In \pref{lem: polyhedron}, we prove that $\mathcal{C}(\Phi_\calX)$ is a union of a finite number of polyhedrons, which implies that it is a closed set since each polyhedron is closed.
	Thus, $\mathcal{C}(\Phi) \cap \{v: \|v\|=1\}$ is closed and bounded. By the extreme value theorem, the minimum element of $\mathcal{S}$ is attainable. Since all elements are positive, we must have $\min_{\epsilon\in\mathcal{S}} \epsilon = C>0$ for some $C$ that is related to $G$ and the feasible set. 
	This finishes the proof.
%	Going back to the first expression of $\mathcal{S}$, the above argument implies that for all $y\in\calY\backslash \calY^*$, 
%	\begin{align*}
%	\max_{x'\in\calV^*(\calX)}    \frac{x^{\prime\top} G(\Pi_{\calY^*}(y)-y)}{\|\Pi_{\calY^*}(y)-y\|} \geq C > 0. 
%	\end{align*}
%	Similarly, 
%\begin{align*}
%	\max_{y'\in\calV^*(\calY)}   \frac{(x-\Pi_{\calX^*}(x))^\top Gy'}{\|x-\Pi_{\calX^*}(x)\|} \geq C'. 
%	\end{align*}
%	
%	Thus, \typeone is satisfied with $\beta=0$. Now it remains to show that $\mathcal{C}(\Phi_\calX)$ or $\mathcal{C}(\Phi_\calY)$ is a closed set. Actually, in the \pref{lem: polyhedron} below, we prove that $\mathcal{C}(\Phi_\calX)$ is a union of a finite number of polyhedrons. Since each polyhedron is a closed set, their finite union is also a closed set. 
	\end{proof}


\begin{lemma}
     \label{lem: deffered lemma}
     The following statements hold (so do the symmetric statements swapping the role of $x$ and $y$): 
     \begin{itemize}
         \item For any $y'\in\calV^*(\calY)$ and any $x^{*}\in\calX^*$, $x^{*\top }Gy'=\rho$. 
         \item There exists $x^{*}\in\calX^*$ such that for all $y'\in\calV(\calY)\backslash \calV^*(\calY)$, $x^{*\top }Gy' < \rho$. 
     \end{itemize}
\end{lemma}
\begin{proof}
     Without loss of generality, we assume $\rho=0$ (otherwise, one can create a new bilinear game $\begin{bmatrix}
         x^\top & 1
     \end{bmatrix}
     \begin{bmatrix}
          G &\mathbf{0} \\
          \mathbf{0} &-\rho
     \end{bmatrix}
     \begin{bmatrix}
           y \\ 1
     \end{bmatrix}
     $ with value $0$ clearly). Also, we transform the game so that it becomes a bilinear game over the simplex (i.e., matrix game): define 
     \begin{align*}
          X = \begin{bmatrix}
               |  & | & \cdots & | \\
               w_1 & w_2 &\cdots & w_{|\calV(\calX)|} \\
               | & | & \cdots & |
          \end{bmatrix}, \qquad 
          Y=\begin{bmatrix}
               |  & | & \cdots & | \\
               v_1 & v_2 &\cdots & v_{|\calV(\calY)|} \\
               | & | & \cdots & |
          \end{bmatrix}
     \end{align*}
     where $\{w_1, \ldots, w_{|\calV(\calX)|}\}$ is the set of vertices of $\calX$, and $\{v_1, \ldots, v_{|\calV(\calY)|}\}$ is the set of vertices of $\calY$. With them, the original bilinear game is equivalent to a matrix game $\bp^\top\hatG\bq$ where $\hatG$ is the following $|\calV(\calX)|\times |\calV(\calY)|$  game matrix: 
     \begin{align*}
         \hatG = X^\top GY. 
     \end{align*}
     and $\bp\in \Delta_{|\calV(\calX)|}$ and $\bq\in \Delta_{|\calV(\calY)|}$. 

     \paragraph{Proving the first statement. }
     By the definition of $\calV^*(\calY)$, if $y'=v_i\in\calV^*(\calY)$, then the following statement is true: 
     there exists $\bq\geq \mathbf{0}$ such that $U\bq\geq  \mathbf{0}$ (element-wise inequality) and $\bb^\top \bq<0$, where
     \begin{align}
          U=\begin{bmatrix}
                \hatG \\
                I_{|\calV(\calY)|\times |\calV(\calY)|} 
          \end{bmatrix}\in \mathbb{R}^{(|\calV(\calX)|+|\calV(\calY)|) \times |\calV(\calY)|}, \qquad \bb=-\be_i.  
     \end{align}     
    where $I_{d\times d}$ denotes the identity matrix of dimension $d$.  This is because there exists a convex decomposition of $y^*=Y\bq$ such that $\bq_i>0$ and $\hatG \bq\geq \mathbf{0}$ (by the optimality of $y^*$). By Farkas's lemma, there does not exist $\br'\geq \mathbf{0}$ such that the following hold simultaneously: 
    \begin{align}
         U^\top \br'=\bb, \qquad \br'\geq \mathbf{0}.  \label{eq: farkas use}
    \end{align}
    We write $\br'= \begin{bmatrix} \bp \\ \br  \end{bmatrix}$, where $\bp\in\mathbb{R}^{|\calV(\calX)|}$ and $\br\in\mathbb{R}^{|\calV(\calY)|}$. Then \pref{eq: farkas use} is same as 
    \begin{align}
         \hatG^\top \bp + \br = -\be_i, \qquad \bp\geq  \mathbf{0}, \quad \br\geq  \mathbf{0}.  \label{eq: farkas use 2}
    \end{align}
    The fact that  \pref{eq: farkas use 2} cannot hold implies that for any $\bp\geq 0$, either there exists $j\neq i$ such that $(\hatG^\top \bp)_j > 0$, or $(\hatG^\top \bp)_i > -1$. 
    
    Let $\bp^*$ be an minimax optimal solution for the game $\hatG$, we know that $(\hatG^\top \bp^*)_j \leq 0$ for all $j$. Therefore, we must have $(\hatG^\top \bp^*)_i > -1$. Suppose that $(\hatG^\top \bp^*)_i\neq 0$ (thus $(\hatG^\top \bp^*)_i < 0$). Then we can always find a large enough constant $M>0$ such that $\bp=M\bp^* \geq \mathbf{0}$ satisfying $(\hatG^\top \bp)_i < -1$ and $\max_{j\neq i} (\hatG^\top \bp)_j \leq 0$ at the same time, which is impossible as discussed. Therefore, the remaining possibility is that $(\hatG^\top \bp^*)_i=0$, which proves the first statement. 
    
    \paragraph{Proving the second statement. } To prove the second statement, we reverse the arguments in the proof for the first statement: let $y'=v_i\in\calV(\calY)\backslash \calV^*(\calY)$, then by the definition of $\calV^*(\calY)$, there does not exists $\bq\geq 0$ such that $U\bq\geq \mathbf{0}$ and $\bb^\top \bq<0$. By Farkas's lemma, there exist $\bp, \br$ such that 
    \begin{align}
         \hatG^\top \bp + \br = -\be_i, \qquad \bp\geq 0, \quad \br\geq 0,   \label{eq: farkas use 3}
    \end{align}
    which implies $(\hatG^\top \bp)_j \leq 0$ for all $j\neq i$ and $(\hatG^\top \bp)_i \leq -1 < 0$. 
    This further indicates that there exists $\bp' \in \Delta_{|\calV(\calX)|}$ such that $(\hatG^\top \bp')_j \leq 0$ for all $j\neq i$ and $(\hatG^\top \bp')_i   < 0$, and consequently $\bp'$ is a minimax optimal solution.

    For each $v_i\in \calV(\calY)\backslash \calV^*(\calY)$ we can follow the above construction and find minimax solution $\bp_i \in \Delta_{|\calV(\calX)|}$ that makes $(\hatG^\top \bp_i)_j \leq 0$ for all $j\neq i$ and $(\hatG^\top \bp_i)_i < 0$. Taking the averaging: $\bp=\frac{1}{|\calV(\calY)\backslash \calV^*(\calY)|}\sum_{i}\bp_i$ we then have $(\hatG^\top \bp)_i< 0$ for all $i$ such that $v_i\in \calV(\calY)\backslash \calV^*(\calY)$. This proves the second statement. 
\end{proof}






\begin{lemma}
	\label{lem: polyhedron}
	Let $\Phi \triangleq \left\{x-\Pi_{\calX^*}(x): x\in \calX\right\}$ and 
	$\mathcal{C}(\Phi) \triangleq \left\{rv: v\in\Phi, r\geq 0\right\}$. If $\calX$ and $\calY$ are polytopes, then $\mathcal{C}(\Phi)$ is a union of a finite number of polyhedrons.    
\end{lemma}
\begin{proof}
	Define for every $x^*\in\calX^*$ the set $\Phi_{x^*}\triangleq \{x-x^*: x\in\calX, \Pi_{\calX^*}(x)=x^*\}$. That is, $\Phi_{x^*}$ consists of $x-x^*$ for all $x\in\calX$ whose projection to $\calX^*$ is $x^*$. Below we derive the form of the conical extension of $\Phi_{x^*}$, i.e., $\mathcal{C}(\Phi_{x^*})=\{r(x-x^*): x\in\calX, \Pi_{\calX^*}(x)=x^*, r\geq 0\}$. 
	
	\paragraph{Claim 1. } If $\calX, \calY$ are polytopes, then $\calX^*$ and $\calY^*$ are also polytopes. 
	\begin{proof}[Proof of Claim 1]
		Note that $\calX^* = \left\{x\in \calX: \max_{y\in\calY} x^\top Gy\leq \rho \right\}$. Since $\calY$ is a polytope, the maximum is attained at vertices of $\calY$. Therefore, $\calX^*$ can be equivalently written as $\left\{x\in \calX: \max_{y\in \calV(\calY)} x^\top Gy\leq \rho \right\}$ where $\calV(\calY)$ is the set of vertices of $\calY$. Since the constraints of $\calX^*$ are all linear constraints, $\calX^*$ is a polytope. 
	\end{proof} 
	
	Now, let $\calX=\{x: Ax-b\leq \mathbf{0}\}$ and $\calX^*=\{x: Ax-b\leq \mathbf{0}, Cx-d\leq \mathbf{0}\}$ for some matrices $A$ and $C$ and vectors $b$ and $d$. The additional constraint $Cx-d\leq \mathbf{0}$ comes from the optimality constraint $\max_{y\in \calV(\calY)} x^\top Gy\leq \rho$. 
	
	Recall from linear programming literature \cite{davis2016a, davis2016b} that the \emph{normal cone} of $\calX^*$ at $x^*$ can be expressed as follows: 
	\begin{align*}
	&\mathcal{N}_{x^*}=\Big\{x-x^*: \ \  x\in\mathbb{R}^M, \quad \Pi_{\calX^*}(x)=x^* \Big\} \\
	&\qquad \qquad = \Big\{ A^\top p + C^\top q: \quad p\geq \mathbf{0}, \quad q\geq \mathbf{0}, \quad p^\top (Ax^*-b)=\mathbf{0}, \quad q^\top (Cx^*-d)=\mathbf{0} \Big\}. 
	\end{align*}
	The normal cone of $\calX^*$ at $x^*$ consists of all outgoing normal vectors of $\calX^*$ originated from $x^*$. It is clear that $\mathcal{C}(\Phi_{x^*})\subseteq \mathcal{N}_{x^*}$ because all vectors in $\mathcal{C}(\Phi_{x^*})$ are outgoing normal vectors from $x^*$. However, it is possible that $\mathcal{C}(\Phi_{x^*})\neq \mathcal{N}_{x^*}$ because the vectors in $\mathcal{C}(\Phi_{x^*})$ has an additional constraint that they are of the form $r(x-x^*)$ for some $x\in \calX$. 
	
	We claim that $\mathcal{C}(\Phi_{x^*})$ is of the following form: 
	\paragraph{Claim 2. }
	\begin{align}
	&\mathcal{C}(\Phi_{x^*}) = \Big\{ A^\top p + C^\top q: \quad p\geq \mathbf{0}, \quad q\geq \mathbf{0}, \quad p^\top (Ax^*-b)=\mathbf{0}, \quad q^\top (Cx^*-d)=\mathbf{0}, \nonumber  \\
	&\qquad \qquad \qquad \qquad a_i^\top(A^\top p+C^\top q)\leq 0 \ \text{\ for all $i$ such that\ } a_i^\top x^*-b_i=0 \Big\}, \label{eq: claim 2}
	\end{align}
	where $a_i^\top$ is the $i$-th row of $A$. 
	
	\begin{proof}[Proof of Claim 2. ]
		\ \\
		``$\subseteq$'': Suppose that $v\in\mathcal{C}(\Phi_{x^*})$. As argued above, $v\in\mathcal{N}_{x^*}$. Therefore, we only need to prove that it satisfies the additional constraint, that is,
		\begin{align*}
		a_i^\top v\leq 0 \ \ \text{for all $i$ such that\ } a_i^\top x^*-b_i=0.  
		\end{align*}
		This is clear when $v=0$. For $v\neq 0$, recall that by the definition of $\mathcal{C}(\Phi_{x^*})$, $v$ can be expressed as $r(x-x^*)$ for some $r > 0$ and $x\in\calX$. Therefore,
		\begin{align*}
		a_i^\top x - b_i 
		&= a_i^\top \left( x^* + \frac{v}{r} \right) - b_i \\
		&= \left(a_i^\top x^* - b_i\right) + \frac{1}{r} a_i^\top v.   
		\end{align*}
		The constraint $x\in\mathcal{X}$ requires that $a_i^\top x-b_i\leq 0$ for all $i$. By the last expression, we see that for all $i$ such that $a_i^\top x^* - b_i=0$, $a_i^\top v\leq 0$ must hold. 
		\ \\
		``$\supseteq$'': Suppose that $v=A^\top p + C^\top q$ is a vector from the set on the right-hand side of \pref{eq: claim 2} where $p$ and $q$ satisfy all the constraints there.  If $v=0$, then clearly, $v\in\mathcal{C}(\Phi_{x^*})$. Below we assume that $v\neq 0$. Consider $x_\epsilon=x^*+\epsilon v$ for some $\epsilon>0$. Notice that 
		\begin{align*}
		p^\top (Ax_\epsilon - b) + q^\top(Cx_\epsilon - d) 
		&= p^\top(Ax^*-b) + q^\top(Cx^*-d) + \epsilon (p^\top A + q^\top C)v \\
		&= 0 +\epsilon \|v\|^2 > 0. 
		\end{align*}
		Since $p\geq 0$ and $q\geq 0$, the above indicates that either $Ax_\epsilon - b\leq \mathbf{0}$ is violated, or $Cx_\epsilon - d\leq \mathbf{0}$ is violated. Therefore, $x_\epsilon \notin \calX^*$. 
		
		Below we show that, on the other hand, when $\epsilon$ is small enough, $x_\epsilon\in\calX$. For all $i$ such that $a_i^\top x^*-b_i=0$, we have
		\begin{align*}
		a_i^\top x_\epsilon - b_i = (a_i^\top x^* - b_i) + \epsilon a_i^\top v \leq 0
		\end{align*}
		by the constraint on $v$ that requires $a_i^\top v\leq 0$. For all $i$ such that  $a_i^\top x^* - b_i < 0$, 
%		\begin{align*}
%		a_i^\top x_\epsilon - b_i = (a_i^\top x^* - b_i) + \epsilon a_i^\top v. 
%		\end{align*}
		%since $ b_i - a_i^\top x^* > 0$, 
		we can always find $\epsilon>0$ small enough so that $\epsilon a_i^\top v \leq b_i-a_i^\top x^*$ and thus $a_i^\top x_\epsilon - b_i = (a_i^\top x^* - b_i) + \epsilon a_i^\top v\leq 0$ for all $i$. 
		
		Thus, we conclude that there is a small enough $\epsilon > 0$ such that $Ax_\epsilon - b \leq 0$, and so $x_\epsilon \in \calX$. Together with the previous arguments, we know $x_\epsilon \in \calX\backslash \calX^*$ and $v$ can be expressed as $\frac{1}{\epsilon}(x_\epsilon-x^*)$. Also, $v\in\mathcal{N}_{x^*}$ implies $\Pi_{\calX^*}(x_\epsilon)=\Pi_{\calX^*}(x^*+\epsilon v)= x^*$. Therefore, $v$ lies in $\mathcal{C}(\Phi_{x^*})$. 	
	\end{proof}
	
	Having identified the form of $\mathcal{C}(\Phi_{x^*})$ for any $x^*$ as \pref{eq: claim 2} (which is a polyhedron), we now argue that there can be only finitely many different $\mathcal{C}(\Phi_{x^*})$ across all $x^*\in\calX^*$. Note that $\mathcal{C}(\Phi_{x^*})$ can be expressed as 
	\begin{align*}
	&\mathcal{C}(\Phi_{x^*}) = \Big\{ A^\top p + C^\top q: \quad p\geq 0, \quad q\geq 0,  \\
	&\qquad \qquad \qquad \qquad p_i=0 \ \text{\ for all $i$ such that\ } a_i^\top x^*-b_i<0 \nonumber  \\
	&\qquad \qquad \qquad \qquad q_i=0 \ \text{\ for all $i$ such that\ } c_i^\top x^*-d_i<0 \nonumber \\
	&\qquad \qquad \qquad \qquad a_i^\top(A^\top p+C^\top q)\leq 0 \ \text{\ for all $i$ such that\ } a_i^\top x^*-b_i=0 \Big\}, 
	\end{align*}
	so $\mathcal{C}(\Phi_x)\neq \mathcal{C}(\Phi_{x'})$ only when the sets of ``tight constraints'' at $x$ and $x'$ are different --- for example, when there exists some $i$ such that $a_i^\top x-b_i < 0$ but $a_i^\top x'-b_i = 0$. Since the total number of constraints is finite, there can only be finitely many different $\mathcal{C}(\Phi_{x^*})$ across all $x^*\in\calX^*$. 
	
	To conclude, $\mathcal{C}(\Phi)$, which by definition is $\bigcup_{x^*\in\calX^*} \mathcal{C}(\Phi_{x^*})$, is a union of finitely many polyhedrons. 
\end{proof}
